# Supplementary material for: Service Function Chaining Simplified
Source: arXiv:1601.00751 source file (2016-01-05)
Supplement: Supplementary file 1 [file appendix.tex]

\section{Linearizing Quadratic Constraint}
\label{section:linearizeQuadraticConstraint}
In this section, we describe how to linearize equations \eqn{throughputConst} and \eqn{bandwidthDemandCons}. 
% We have to linearize the multiplication of $y_{vn}(x_{uv}^{mn} + x_{uv}^{nm})$. 
Let define two slack variables as in \eqn{slackVariable1} and \eqn{slackVariable2}:
\begin{equation}
\small
\begin{aligned}
    &\forall n \in N:
        \forall (m,n) \in L_n, m < n:
            \forall v \in \mathcal{N}:
                \forall (u,v) \in \mathcal{L}_{v}^{in}: \\
                    &z_{uv}^{mn} = 
                        \begin{cases}
                            x_{uv}^{mn} &  \mbox{if } y_{vn} = 1\\
                            0           &  \mbox{if } y_{vn} = 0
                        \end{cases}
\end{aligned}
\label{equation:slackVariable1}
\end{equation}
\begin{equation}
\small
\begin{aligned}
    &\forall n \in N:
        \forall (m,n) \in L_n, m < n:
            \forall v \in \mathcal{N}:
                \forall (v, u) \in \mathcal{L}_{v}^{out}: \\
                    &\hat{z}_{vu}^{mn} = 
                        \begin{cases}
                            x_{vu}^{mn} &   \mbox{if } y_{vn} = 1\\
                            0           &   \mbox{if } y_{vn} = 0
                        \end{cases}
\end{aligned}
\label{equation:slackVariable2}
\end{equation}

To achieve above definitions constraints in \eqn{slackVariablesConst} have to be satisfied. For the sake of simplicity we remove the subscripts and superscripts. The first two inequalities ensure that if $y=0$, then $z=0$. The second two inequalities assures than if $y=1$, then $z=x$. $\Gamma \in \mathbb{R^+}$ is a big enough number.
\begin{equation}
\small
\label{equation:slackVariablesConst}
    \begin{aligned}
        z   &\leq   \Gamma y
        &,
        z   &\geq   0                \\
        z   &\leq   x
        &,
        z   &\geq   x - (1-y) \Gamma
    \end{aligned}
\end{equation}

Thus, \eqn{throughputConst} is revised as \eqn{reThroughputConst}:
\input{equations/reThroughputConst}

Finally, \eqn{bandwidthDemandCons} is rewritten as \eqn{reBandwidthDemandCons}:
\input{equations/reBandwidthDemandCons}
